# Supplementary material for: ESG: Elastic Graphs for Range-Filtering Approximate k-Nearest Neighbor Search
Source: arXiv:2504.04018 source file (2025-04-05)
Supplement: Supplementary file 1 [file appendix.tex]

\newpage
\appendix
\section{Appendix}

\subsection{Proofs}
\stitle{Proof of Lemma~\ref{lem:top-k}.}
    From the definition~\ref{def:rfanns} of range-filtering $k$ nearest neighbor search, the range-filtering $k$ nearest neighbor set $S_k$ of a query $q$ with filter $[l,r]$ consists of the $k$ nearest neighbors within $[l,r]$, these points are, by definition, closer (in terms of the distance metric) than any other points within $[l,r]$ not in $S_k$. Given that $S_r$ is the set of the top-$r$ nearest neighbors overall, and it contains at least $k$ points within $[l,r]$, these $k$ points must be among the $r$ nearest overall points. Next, we prove this problem by contradiction. If there were a point in $S_k$ that was not in $S_r$, it would imply that there exists a closer point (since $S_r$ already includes the top $r$ nearest neighbors). However, this contradicts the assumption that $S_k$ contains the $k$ nearest neighbors within the range. Therefore, all points in $S_k$ must be included in $S_r$ to satisfy both the range condition and the nearest neighbor condition.

\stitle{Proof of Theorem ~\ref{thm:KNN-time-complexity}.}
    The author of~\cite{DBLP:journals/pvldb/NSGFuXWC19} discusses the search time complexity of nearest neighbor search. However, there is no direct statement of the top $k$ nearest neighbor search time complexity. Recall that with the same assumption in~\cite{DBLP:journals/pvldb/NSGFuXWC19}, the Algorithm~\ref{alg:graph-search} finds the top 1 nearest neighbor with the expected length 
\begin{equation*}
    O(\frac{N^{\frac{1}{d}} \log N^{\frac{1}{d}}}{\bigtriangleup r}).
\end{equation*}
    Then we get the top $k$ nearest neighbor search time complexity based on the reduction method and the property of MSNET~\ref{def:MSNET}. Consider we find the top $1,...,k-1$ nearest neighbor $v_1,..,v_{k-1}$ of $q$ and search for the top $k$-th nearest neighbor $v_k$. From the property of MSNET, any two points have a monotonic search path. The $v_k$ and $q$ are connected by a monotonic search path with the same expected length. Then, the expected search path length of the top $k$ nearest neighbor search will be
\begin{equation*}
    O(k\times\frac{N^{\frac{1}{d}} \log N^{\frac{1}{d}}}{\bigtriangleup r}).
\end{equation*}

From the above time complexity, we can find that theoretically, the time cost of searching top-$K$ neighbors should be $k$ times that of top-1. However, in practice, we found that the time cost of searching top-$k$ neighbors by algorithms such as HNSW and NSG is far less than $k$ times that of top-1. Meanwhile, even if there exists $k$ monotonic search path from the query to its $k$ nearest neighbor. It is still hard for Algorithm~\ref{alg:graph-search} to strictly follow the search path since the top $k$ nearest neighbor can not be identified before reached.
However, we found that the existing graph index such as HNSW and NSG will reversely connect its neighbor to the current point (reverse edge) after edge occlusion.

Then, we reconsider the property of MSNET. From the definition of MSNET, the $v_k$ is either connected to $q$ or a monotonic search path $v_k,v^{\prime},...,q$ exists and $||v_k,q|| > ||v^{\prime},q||$
Because $v_k$ is the top $k$ nearest neighbor of $q$, then $v^{\prime}$ must be one of $v_1,...,v_{k-1}$ which is already visited. However, the edge from $v_k$ to $v^{\prime}$ is a directed edge. Even though we have visited $v^{\prime}$, we still cannot directly access $v_k$. After adding the reverse edges of all outgoing edges of $v_k$, we can directly access $v_k$ through the reverse edge from $v_k$ to $v^{\prime}$. (Adding additional edges does not affect the property of MSNET, that is, the monotonic search path between two points still exists.)
    
From Algorithm~\ref{alg:graph-search} the neighbor of visited points are pushed into the candidate queue $C$. If the top $1,...,k-1$ nearest neighbor is found, then $v_k$ will be at the top of the candidate queue and only 1 extra step is needed. Then we can derive that the expected search path length of MSNET for the top $k$ nearest neighbor is:
    \begin{equation*}
        O(\frac{N^{\frac{1}{d}} \log N^{\frac{1}{d}}}{\bigtriangleup r} + k)
    \end{equation*}
where only an extra $k$ step is needed.

\stitle{Proof of Theorem ~\ref{thm:half-blood-search-time-complexity}.}
    With the conclusion in Lemma~\ref{lem:top-k} and Theorem~\ref{thm:KNN-time-complexity}, the expected search path of an MSNET with reverse edge finds the range-filtering nearest neighbor can be regarded as the expected path length that accumulates \textit{in-range} $k$ nearest neighbor. Note that we only consider cases where $k$ is less than the range filter size. The RFKNN only exists in such a setting. Specifically, we regard the top $h$ nearest neighbor search as a drawing problem without replacement. Starting from the search for the top $k$ nearest neighbor, each search for the $k$+1th nearest neighbor can be regarded as drawing one from $N$ data points, where the \textit{in-range} point is considered a success and the out-range point is considered a failure. In this way, the extra steps of implementing the top-$k$ range filtering nearest neighbor search through the top-$h$ nearest neighbor search can be regarded as the expected number of drawing times to accumulate a total of $k$ \textit{in-range} points.

    Formally, we set $N$ as the overall number of points, $K$ as the \textit{in-range} number of points, and $L$ as the \textit{out-range}. Our target is to find the expected number of draws $E[T]$ when the $k$-th \textit{in-range} point is drawn. To find $E[T]$, we can use the method of order statistics, that is, consider the expected position of the $k$-th \textit{in-range} in the number of draws among all possible arrangements of the index visited points.

    With the assumption in~\cite{DBLP:journals/pvldb/NSGFuXWC19} and the attribute values of points in $\mathcal{D}$ are independent. That is, for any $i\in[1,N]$, each point in $\mathcal{D}$ appears in the $i$-th position of the ordering of $\mathcal{D}$ with an equal probability. Then, assume that all $N$ points are randomly arranged with equal probability. We are interested in the position of the range-filtered $k$ nearest neighbors in this arrangement(sorted by distance to query $q$). Let the position of $k$ range-filtered nearest neighbor be $W_1<W_2<W_3,...,<W_k$. Our goal is to find the expectation of $W_k$ the $E[W_k]$.

    In the case of discrete uniform distribution, the expectation of the order statistic of the sequence position can be calculated by combinatorial methods.
    We first consider the total number of permutations. Select $K$ positions from $N$ positions to place the \textit{in-range} point. There are $\binom{N}{K}$ options. For the number of cases where the $k$-th \textit{in-range} point ($k$-th range filtering nearest neighbor) is at position $i$: There must be $k$-1 in-range points in the first $i$-1 positions, position $i$ is the $k$-th \textit{in-range} point, and there are $K$-$k$ \textit{in-range} points in the remaining positions $N-i$. Therefore, the number of permutations that meet the conditions is $\binom{i-1}{k-1}\binom{N-i}{K-k}$.

    According to the definition of expectation:
    \begin{equation*}
        E[W_k]=\sum\limits_{i-k}^{N-K+k}i\times\frac{\binom{i-1}{k-1}\binom{N-i}{K-k}}{\binom{N}{K}}
    \end{equation*}
    Note that an important identity for the number of combinations is:
    \begin{equation*}
        i\binom{i-1}{k-1}=k\binom{i}{k}
    \end{equation*}
    Substituting the above identity into the original expression we get:
    \begin{equation*}
    \begin{aligned}
        E[W_k] & =\frac{1}{\binom{N}{K}}\sum_{i=k}^{N-K+k}i\binom{i-1}{k-1}\binom{N-i}{K-k}\\ 
         &=\frac{1}{\binom{N}{K}}\sum_{i=k}^{N-K+k}k\binom{i}{k}\binom{N-i}{K-k}\\
         &=\frac{k}{\binom{N}{K}}\sum_{i=k}^{N-K+k}\binom{i}{k}\binom{N-i}{K-k}
    \end{aligned}
    \end{equation*}
    We next calculate the summation term. Note the following combinatorial identity (a variation of the Vandermonde's identity)
    \begin{equation*}
        S=\sum_{i=0}^{N}\binom{i}{k}\binom{N-i}{K-k}=\binom{N+1}{K+1}
    \end{equation*}
    Since in our summation, the number of combinations is zero when $i<k$ or $i>N-(K-k)$, the upper and lower limits of the summation can be extended to $i=0$ to $N$ without affecting the result.
    Therefore, we have:
    \begin{equation*}
    \begin{aligned}
        E[W_k]&=\frac{k}{\binom{N}{K}}\binom{N+1}{K+1}\\
              &=k \times \frac{N+1}{K+1}
    \end{aligned}
    \end{equation*}
    Under the condition of satisfying elastic factor constraint, that is, $K \geq N \times c$, we further simplify the formula:
    \begin{equation*}
    \begin{aligned}
        E[W_k]&\leq k\times\frac{N+1}{N\times c+1}=O(k/c)
    \end{aligned}
    \end{equation*}
    So far, we have proved that the expected number of additional steps to search for the Top $k$ range filtering nearest neighbor is $O(k/c)$. We take $N^{\prime}=|[L,R]|$, then the final expected search length can be written as:
    \begin{equation*}
    O(\frac{N^{\prime\frac{1}{d}} \log N^{\prime\frac{1}{d}}}{\bigtriangleup r^{\prime}} +k/c)
    \end{equation*}
    where $O(k)$ for extra step for top $k$ RFKNN search.

\stitle{Proof of Lemma~\ref{lem:worse-2-index-select}.}
    We first find the corresponding segment tree node according to the segment tree split method. That is, if the ranges corresponding to the query and the right subtree overlap, then we directly access the right subtree, and the same goes for the left subtree. If the query range overlaps with the range of left and right subtrees of the current tree node, we first determine whether the current node satisfies the elastic factor constraint. If so, we use the graph index corresponding to the current node to perform the $\POST$ algorithm, that is, only one index is used. If the query does not satisfy the elastic factor constraint, we split the range filter $[l,r]$ of the query into $[l, mid]$ and $[mid, r]$ respectively. After splitting, we can convert the general query into two half-bounded queries with range filter $[l,mid]$ and $[mid,r]$. Let $[L,R]$ be the current segment tree range, and $[l,mid] \subseteq [L,mid]$ and $[mid,r] \subseteq [mid,R]$. For the query with filter $[l,mid]$. We only traverse the right subtree of the current node and the next node and determine whether it meets the elastic factor constraint. Each time we traverse the right subtree, the overall interval will be shortened by half, while the right bound remains unchanged. This search strategy is the same as the $\HBIO$ index, and only one index is needed in the end. Similarly, the range filter $[mid,r]$ also only needs one index. Then we can prove that the $\HBIT$ index uses two indexes for general queries in the worst case.

\stitle{Proof of Lemma~\ref{lem:worse-f-index-select}.}
    Let $f$ denote the fanout of the segment tree, the elastic factor constraint is $1/f$. If the query range $[l,r]$ requires more than or equal to 3 subtrees to cover, then the middle index range will be completely covered by the query range. Let $[l_m,r_m]$ be one of the middle index ranges and $[l_r,r_f]$ be the father node index range. The elastic factor of $e([l_m,r_m],[l_m,r_m]$ will be equal to $1/f$. Since, $[l_q,r_q]$ cover $[l_m,r_m]$ and be covered by $[l_f,r_f]$, the elastic factor will greater than $1/f$. Then the father range index $[l_f,r_f]$ can be invoked for RFANN search which only uses one index.  If the query range $[l,r]$ requires 2 subtrees to cover, we use the same split strategy to convert the general RFAKNN query into two half-bounded queries. Then only two indexes are used. If the query range can be covered by only one subtree, we follow the segment tree search strategy to keep searching.

\subsection{Discussion}
\stitle{Discussion of Modular Graph Index.}
Our algorithms, $\HBIO$, and $\HBIT$, serve as frameworks with the default graph indexing algorithm set to $\HNSW$, due to its widespread application and robust performance. It is worth noting that replacing the $\HNSW$ algorithm with more advanced algorithms like $\tau$-MG~\cite{tMRNG:journals/pacmmod/PengCCYX23} or VAMANA~\cite{Diskann-NIPS-2019} might improve time complexity or practice search efficiency. However, while $\tau$-MG offers better search time complexity, it incurs a larger out-degree for each node at $O(\log N)$, which leads to a higher spatial cost for the $O(\log N)$ layers required by $\HBIT$. Meanwhile, $\HNSW$ supports continuous insertions, and we have significantly optimized index construct efficiency based on this feature.

Another solution to the problem of memory pressure caused by a large graph index is the disk AKNN search solution~\cite{Diskann-NIPS-2019,Starling-SIGMOD-2024-Mengzhao}. In the graph-based disk search scenario, only the compressed vectors are stored in memory, and the full-precision vectors and graph indexes are stored on disk. For the $\HBIT$ algorithm that requires a large memory space for storage, the graph structure is placed on the disk as the main space cost, so the memory cost is the same as the original disk-based graph-index methods that is, only the compressed vector is in memory.

\subsection{Additional Experimental Results}

\stitle{Exp-A.1. Test of Varying Range Lengths on Half-Bound Queries.}
\input{figure/half-result}
We provide a variety of half-bounded range filter search performance tests in Fig.~\ref{fig:half-range-filter-results-all}. Note that the use of a range filter from $[1,N/2^i]$ will lead to the $\HBIO$ algorithm having the theoretical optimal performance since the elastic factor will be 1. From the experiment result, our algorithm has a stable performance improvement relative to the $\SERF$ algorithm cross various range filters.

\stitle{Exp-A.2. Additional Experiments on Large-Scale Data.}
\input{figure/large-scale-fanout}
For large-scale data, the indexing time and index space are typically large. 
A simple method is to use a segment tree with a larger fanout to reduce the number of index layers. The consequence of a larger fanout is a reduction in search performance. Therefore, we conducted additional experiments. 
As shown in Fig.~\ref{fig:large-results-fanout}, we compared the cases of fanout set as 2 ($\HBIT$-2), and fanout set as 16 ($\HBIT$-16). 
It can be seen that both settings can achieve a high search recall. 
Also, the performance gap between the two fanout settings is not significant at a high recall level. However, at a lower recall level, $\HBIT$-2 has a 2x-6x performance advantage over $\HBIT$-16. However, $\HBIT$-2 requires 2x the build time and 3x the time cost of $\HBIT$-16. Therefore, for a scenario with limited index memory space and build time, a $\HBIT$ with a large fanout, such as 16, can be adapted.
